# Supplementary material for: The Effects of Adding Reachability Predicates in Quantifier-Free Separation Logic
Source: arXiv:1810.05410 source file (2021-02-28)
Supplement: Supplementary file 1 [file appendix.tex]

This technical appendix contains the proofs omitted  from the body of the paper.
Intermediate lemmas are added and new notations and definitions are provided.

\OnlyForVL{
\subsection{Proof of Lemma~\ref{lemma-meet-unique}}

 \input{proof-meet-unique}
}

%%\section{Proof of Lemma~\ref{lemma-labels}}

%% \input{proof-lemma-labels-subset}

\section{$\seplogic{\separate, \reachplus}$ and other \pspace variants}

\subsection{Proof of Lemma~\ref{lemma-atomic-formulae-test}}

 \input{proof-lemma-atomic-formulae-test}%%

%%
%% \section{Proof of Lemma~\ref{lem:sees}}
%%
%% \input{proof-lemma-sees}
%%

\subsection{Introduction to support graphs}
%\label{appendix-support-graph}%%
In order to prove Lemma~\ref{lemma-star} (see Appendix~\ref{appendix-proof-lemma-star}),
we introduce the notion support graph and show its main properties.
Given a memory state  $\pair{\astore}{\aheap}$ and $q \geq 1$, below we define the notion of
support graph $\supportgraph{\astore,\aheap}$ that is a structure that records all the properties
of the memory state  $\pair{\astore}{\aheap}$ that are useful to check the satisfaction of each
test formula from $\Test(q,\alpha)$. Even though $\supportgraph{\astore,\aheap}$ simply reorganises
the properties of $\pair{\astore}{\aheap}$, it will be helpful as isomorphic supports graphs
(with the adequate notion of isomorphism) witness that the underlying memory states satisfy
the same test formulae.

\begin{definition}
  Let $q \geq 1$ and $\pair{\astore}{\aheap}$ be a memory state.
  The \defstyle{support graph} $\supportgraph{\astore,\aheap} = (\gverts,\gedges,\galloc,\glabels,\gbtw,\grem)$
is defined as follows:
  \begin{itemize}
  \itemsep 0 cm
  \item $\gverts \egdef \Labels{q}{\astore,\aheap}$;
  \item $\gedges$ is a functional binary relation on $\gverts$
        such that $\pair{\alocation}{\alocation'} \in \gedges$ $\equivdef$
        there is $L \geq 1$ such that $\aheap^{L}(\alocation) = \alocation'$ and for all $0 < L' < L$,
        it holds that $\aheap^{L'}(\alocation) \not \in \gverts$;
    \item $\galloc \egdef \gverts \cap \domain{\aheap}$;
    \item $\glabels: \gverts \to \powerset{\Terms{q}}$ such that for all $\alocation \in \gverts$,
    $\glabels(\alocation) \egdef \invsem{\alocation}{q}{\astore,\aheap}$ where
    $$
    \invsem{\alocation}{q}{\astore,\aheap} \egdef \set{\aterm \in \Terms{q} \ \mid \ \sem{\aterm}^q_{\astore,\aheap} = \alocation}
     ;
    $$
    \item $\gbtw: \gedges \to \powerset{\locations}$ such that for all $\pair{\alocation}{\alocation'} \in \gedges$,
    \begin{gather*}
    \gbtw(\alocation,\alocation') \egdef
    \left\{
    	\alocation''\
   		\middle|
    \begin{aligned}
    	\text{there are } L,L' \geq 1\ \aheap^{L}(\alocation) = \alocation'' \text{ and } \aheap^{L'}(\alocation'') = \alocation'\\
    	\text{ and for all } L'' \in [1,L]\ \aheap^{L''}(\alocation) \not\in V
    \end{aligned}
    \right\}
   	\end{gather*}
    \item $\grem \egdef \Others^q_{\astore,\aheap}$.
  \end{itemize}
\end{definition}
 Support graphs abstract the properties of memory states for  checking the satisfaction of
test formulae. As an illustration, the semantics for the test formulae can be easily reformulated
with the help of  support graphs.%%
\begin{align*}
 \pair{\astore}{\aheap} &\models \aterm = \aterm ' && {\rm iff} && \sem{\aterm}^q_{\astore,\aheap}
 \in V  \ {\rm and} \ \set{\aterm, \aterm'} \subseteq \glabels(\sem{\aterm}^q_{\astore,\aheap}) \\
  \pair{\astore}{\aheap} &\models \alloc{\aterm} && {\rm iff}  && \astore(\aterm) \in \galloc \\
  \pair{\astore}{\aheap} &\models \aterm \hpto \aterm' && {\rm iff}  && \alocation = \sem{\aterm}^q_{\astore,\aheap}, \alocation' =
\sem{\aterm'}^q_{\astore,\aheap}
 \in V  \ {\rm and} \ \\
 &&&&& \pair{ \alocation}{ \alocation'} \in \gedges  \ {\rm and} \
        \card{\gbtw( \alocation, \alocation')} = 0 \\
 \pair{\astore}{\aheap} &\models \sees_q(\aterm,\aterm') \geq \beta +1 && {\rm iff}  &&
 \alocation = \sem{\aterm}^q_{\astore,\aheap},
 \alocation' = \sem{\aterm'}^q_{\astore,\aheap} \in V,   \\
 &&&&& \pair{ \alocation}{ \alocation'} \in \gedges  \ {\rm and} \ \card{\gbtw( \alocation, \alocation')} \geq \beta \\
  \pair{\astore}{\aheap} &\models \sizeothers_q \geq \beta &&  {\rm iff} && \card{\grem} \geq \beta
\end{align*}

This definition of support graphs is useful since it highlights the information that can be checked via
test formulae. As such, the following lemma holds.

\begin{lemma}
  Let $q,\alpha \geq 1$ and $\pair{\astore}{\aheap}$ and $\pair{\astore'}{\aheap'}$ be two memory states and let
$(\gverts,\gedges,\galloc,\glabels,\gbtw,\grem)$ and $(\gverts',\gedges',\galloc',\glabels',\gbtw',\grem')$ be their respective
support graphs with respect to $q$.
We have $\pair{\astore}{\aheap} \approx^q_\alpha \pair{\astore'}{\aheap'}$ iff there is a map $\amap:  \gverts \to \gverts'$
such that
  \begin{enumerate}[label=\textbf{(A\arabic*)}]
  \itemsep 0 cm
  \item $\amap$ is a graph isomorphism between $\pair{\gverts}{\gedges}$ and  $\pair{\gverts'}{\gedges'}$,
  \item for all $\alocation \in \gverts$, we have $\alocation \in \galloc$ iff  $\amap(\alocation) \in \galloc'$,
  \item for all $\alocation \in \gverts$, $\glabels(\alocation) = \glabels'(\amap(\alocation))$,
  \item for all  $\pair{\alocation}{\alocation'} \in \gedges$,
       \[\min(\alpha,\card{\gbtw(\alocation,\alocation')}) = \min(\alpha,\card{\gbtw'(\amap(\alocation),\amap(\alocation'))}),\]
   \item $\min(\alpha, \card{\grem}) = \min(\alpha, \card{\grem'})$.
 \end{enumerate}
\end{lemma}%%

\input{proof-lemma-test-graph}

%% \section{Proof of Lemma~\ref{lemma-test-graph}}
%%
%% \input{proof-lemma-test-graph}
%%

\subsection{A lemma about labels}

Before proving Lemma~\ref{lemma-star} we need the following intermediate result, stating that labelled locations cannot be introduced by removing memory cells of a heap.

%\label{labels-lemma}
\begin{lemma}
%\label{lemma-labels}
Let $\pair{\astore}{\aheap}$ be a memory state, $\aheap' \sqsubseteq \aheap$ and $q \geq 1$. It holds
that $\Labels{q}{\astore, \aheap'} \subseteq \Labels{q}{\astore,\aheap}$.
\end{lemma}%%
\input{proof-lemma-labels-subset}

\subsection{Proof of Lemma~\ref{lemma-star}}
%\label{appendix-proof-lemma-star}

 \input{proof-lemma-star}

\subsection{Proof of Theorem~\ref{theorem-quantifier-elimination}(I)}

 \input{proof-theo-test-sl-equiv}

\subsection{Proof of Theorem~\ref{theorem-quantifier-elimination}(II)}

 \input{proof-theorem-quantifier-elimination}%%

\subsection{Proof of  Theorem~\ref{theorem-finite-heap-property}}

 \input{proof-theorem-finite-heap}

In the following proofs, let $\acompmap(N,M) \egdef (N^2 + N)(M+1) + M$.

\subsection{Proof of Theorem~\ref{theorem-pspace}}

 \input{proof-theorem-pspace}

\subsection{Proof Sketch of Corollary~\ref{corollary-bool-shf}}

Our developments for  $\seplogic{\separate, \reachplus}$ allow us to get the \np upper bound as a
by-product and this is done thanks to
an alternative proof based on the test formulae. Note that in the formulae below, the separating conjunction $\separate$
cannot occur in the scope of negation.
Actually, this bound applies to the positive fragment of  $\seplogic{\separate, \reachplus}$ in which negation occurs
 only in front of atomic formulae.
Let us briefly define the SHF formulae $\aformula$ as conjunctions $\apureformula \wedge \aspatialformula$
where $\apureformula$ is a
\defstyle{pure formula} and $\aspatialformula$ is a \defstyle{spatial formula} $\aspatialformula$:
$$
\apureformula ::= \perp  \ \mid \ \top  \ \mid \ (\avariable_i = \avariable_j) \ \mid \  \neg (\avariable_i = \avariable_j) \ \mid \
\apureformula \wedge \apureformula
$$
$$
\aspatialformula ::= \emptyconstant \ \mid \ \top \ \mid \ \avariable_i \mapsto \avariable_j \ \mid \ \ls(\avariable_i,\avariable_j) \ \mid \
\aspatialformula \separate \aspatialformula \ \ \ \ \ \ \ \
\aformula ::= \apureformula \wedge \aspatialformula
$$
Obviously, $\avariable_i \mapsto \avariable_j$ is interpreted as the exact points-to relation.

\input{proof-corollary-bool-shf}

\subsection{Proof  of Theorem~\ref{theorem-boolean-combination}}

\input{proof-theorem-boolean-combination}

\subsection{Proof of Theorem~\ref{theorem-last-decidability}}

 \begin{proof}
Let $\aformula$ be a formula in $\seplogic{\separate, \magicwand, \reachplus}$ in which $\reachplus$ is not
in the scope of $\magicwand$ 
and the program variables are among $\avariable_1$, \ldots, $\avariable_q$. The algorithm works as follows.
\begin{enumerate}
\itemsep 0 cm
\item For each maximal subformula $\aformulabis$ of $\aformula$ whose main connective is $\magicwand$ (and therefore
$\aformulabis$ is in $\seplogic{\separate, \magicwand}$), we compute a Boolean combination of test formulae
from those mentioned in Proposition~\ref{proposition-prop-sl}.  Actually Proposition~\ref{proposition-prop-sl} states
its existence but we can restrict ourselves to test formulae among 
$\size \geq \beta$ with $\beta \leq 2 \length{\aformula}$, $\alloc{\avariable_i}$,
$\avariable_i \pointsl{} \avariable_j$ and $\avariable_i = \avariable_j$ ($i,j \in \set{1,\ldots,q}$). 
One can enumerate the non-equivalent Boolean combinations $\aformulater$ built on those test formulae
and check in polynomial space in $\length{\aformulater} + \length{\aformulabis}$ whether
$\aformulater \Leftrightarrow \aformulabis$ is valid. Indeed, the validity problem for
$\seplogic{\separate, \magicwand}$ is in \pspace~\cite{Calcagno&Yang&OHearn01}. The enumeration
can be done in exponential space as well as the validity checking. 
\item  Let $\aformula'$ be the formula in  $\seplogic{\separate, \reachplus, \bigcup_{q,\alpha} \Test(q,\alpha)}$ obtained
       from $\aformula$ by replacing every maximal subformula $\aformulabis$  whose main connective is $\magicwand$
       by its equivalent Boolean combination with test formulae from $\Test(q,  2 \length{\aformula})$ by using  
       also Lemma~\ref{lemma-atomic-formulae-test} to eliminate the atomic formula of the form $\size \geq \beta$. The size of $\aformula'$ is exponential in $\length{\aformula}$
       and $\aformula'$ can be computed in exponential space in $\length{\aformula}$.
\item  Since the satisfiability problem for $\seplogic{\separate, \reachplus, \bigcup_{q,\alpha} \Test(q,\alpha)}$
       is in \pspace when the constants are encoded in unary and the maximal constant in  $\aformula'$ is $2 \length{\aformula}$,
       the satisfiability status of $\aformula'$ can be checked in polynomial space in $\aformula'$ and therefore
       in exponential space in $\length{\aformula}$. 
\end{enumerate}
Hence, the satisfiability problem is decidable and in \expspace according to the analysis above. \qed 
\end{proof}
